# Supplementary material for: DisCo RL: Distribution-Conditioned Reinforcement Learning for General-Purpose Policies
Source: arXiv:2104.11707 source file (2021-04-23)
Supplement: Supplementary file 2 [file 8_appendix_short.tex]

\section{Generalization to Real-World Robots}\label{appsec:real-world-robot}
While our experiments were only conducted in simulated environments, we expect \METHOD to generalize to real-world robots.
We note that both goal-conditioned RL~\citep{nair2018rig} and VICE~\citep{singh2019raq} have been applied to real-world robot domains, and that \autoref{fig:long-horizon-results} demonstrates that \METHOD can significantly outperform these methods in multi-task settings where tasks are not specified by single goals.
We note that these findings are consistent across all three simulated domains, suggesting that these results are general properties of the methods and may apply to other domains, including real-world robotics.
We also note that the PyBullet
simulator~\cite{coumans2013bullet} has been successfully applied for sim-to-real transfer~\citep{tan2018quadruped,peng2020learning}, suggesting that strong performance in the simulator can generalize to real-world robots.

Lastly, in our experiments \METHOD used $30$ to $50$ examples to learn goal distributions that specify different robot tasks.
Specifying such few number of example successful states is particularly practical for real-world domains, where specifying tasks often requires manually specifying reward functions or adding task-specific instrumentation and sensors. 

\section{Environments}\label{appsec:env-details}
\paragraph{Sawyer}
This environment is based in the PyBullet~\cite{coumans2013bullet} physics simulator.
It consists of a Sawyer robot mounted next to a table, on top of which there is a tray and four blocks.
The robot must learn to manipulate the blocks via its gripper.
The robot is controlled via position control, and it is restricted to move in a 2D plane.
Specifically, the robot arm can move in the YZ coordinate plane and the gripper can open along the X axis, where the X, Y, Z axes move along the front-back, left-right, and up-down directions of table, respectively.
We also constrain the objects to move along the YZ coordinate plane.
The agent has access to state information, comprising of the position of the end effector and gripper state, as well as the positions of the objects and tray.

\paragraph{Visual Sawyer}
We use the same environment as described above for the vision-based tasks but replace the state with 48x48 RGB images.
We pretrain a VAE on 5120 randomly generated images and obtain the goal distribution using 30 example images.
We visualize some example images in \Cref{fig:example-images}.

The encoder consist of a 3 convolutions with the following parameters
\begin{enumerate}
    \item channels: 64, 128, 128
    \item kernel size: 4, 4, 3
    \item stride: 2, 2, 2
    \item padding: 1, 1, 1
\end{enumerate}
followed by 3 residual layers each containing two convolutions with the following parameters
\begin{enumerate}
    \item channels: 64, 64
    \item kernel size: 3, 1
    \item stride: 1, 1
    \item padding: 1, 1
\end{enumerate}
and two linear layers that projects the convolution output into the mean and log-standard deviation of a Gaussian distribution in a latent dimension with dimension 64.

The decoder begins with a linear layer with the transposed shape as the final encoder linear layer, followed by a reshaping into a latent image the same shape as the final encoder convolution output shape.
This latent image is put through a convolution (128 channels, kernel size 3, stride 1, padding 1), and then an equivalent residual stack as the encoder, and two transposed convolutions with parameters
\begin{enumerate}
    \item channels: 64, 64
    \item kernel size: 4, 4
    \item stride: 2, 1
    \item padding: 2, 1
\end{enumerate}
which outputs the mean of a Gaussian distribution with a fixed unit variance.
We trained this VAE with Adam with a learn rate of $10^{-3}$ and default PyTorch~\citep{pytorch2019} parameters ($\beta_1 =0.9$ and $\beta_2 = 0.999$) for 100 epochs and annealed the loss on the KL term from 0 to 1 for the first 20 epochs.

\begin{figure}[h]
    \centering
    \includegraphics[height=2.2cm]{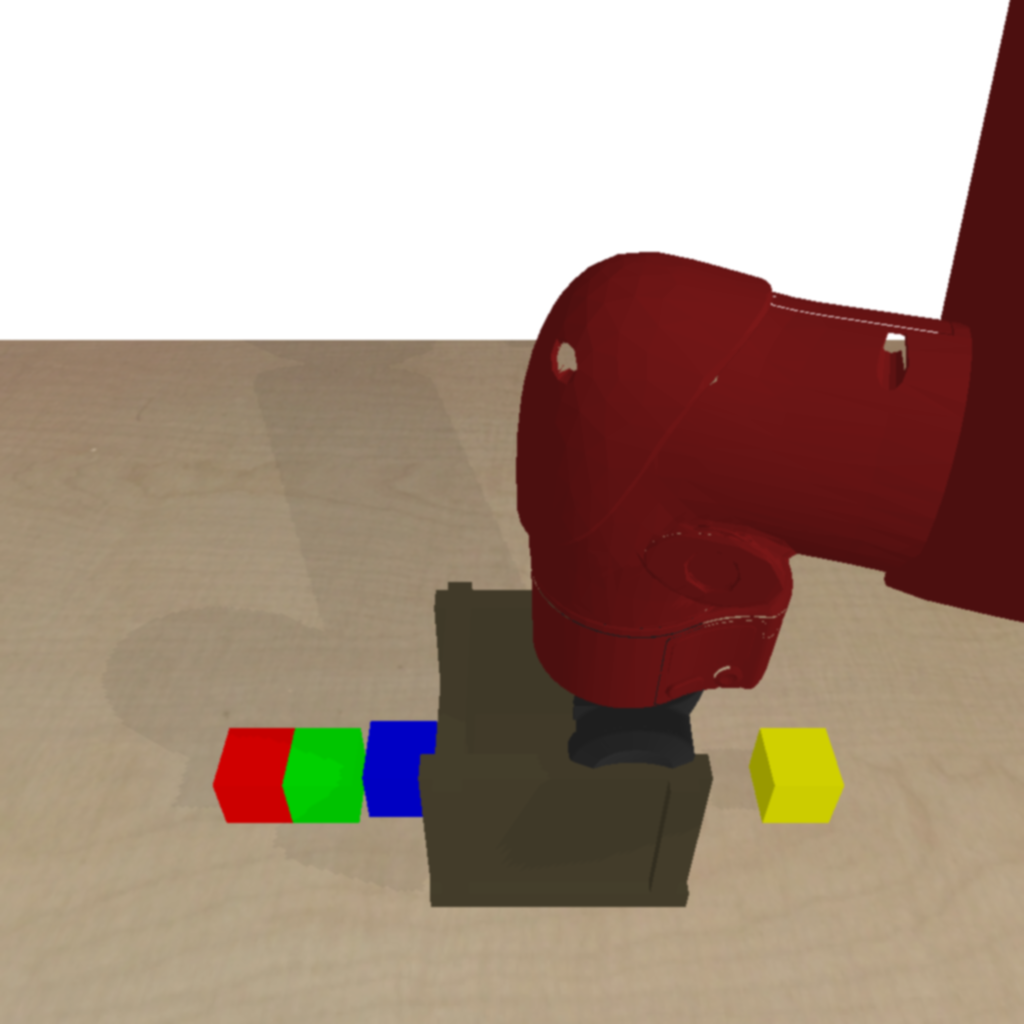}
    \hfill
    \includegraphics[height=2.2cm]{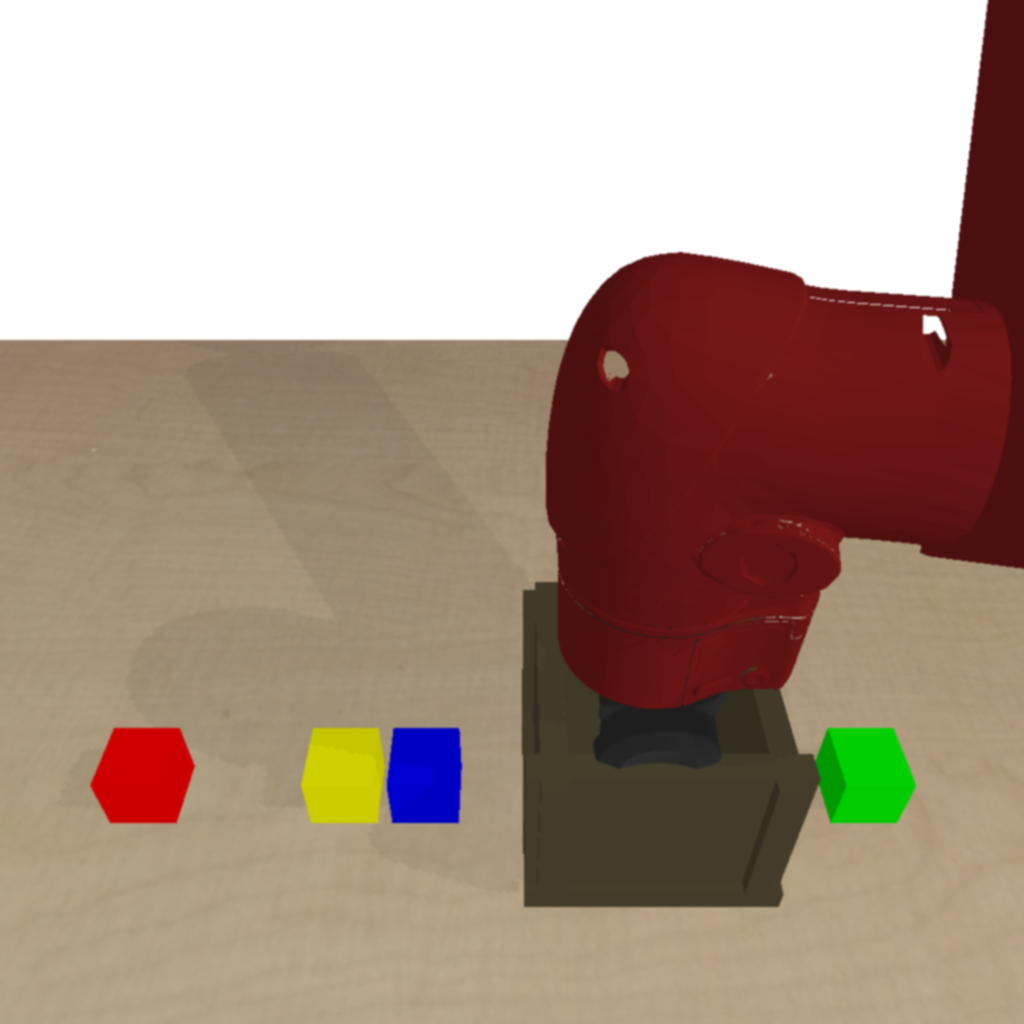}
    \hfill
    \includegraphics[height=2.2cm]{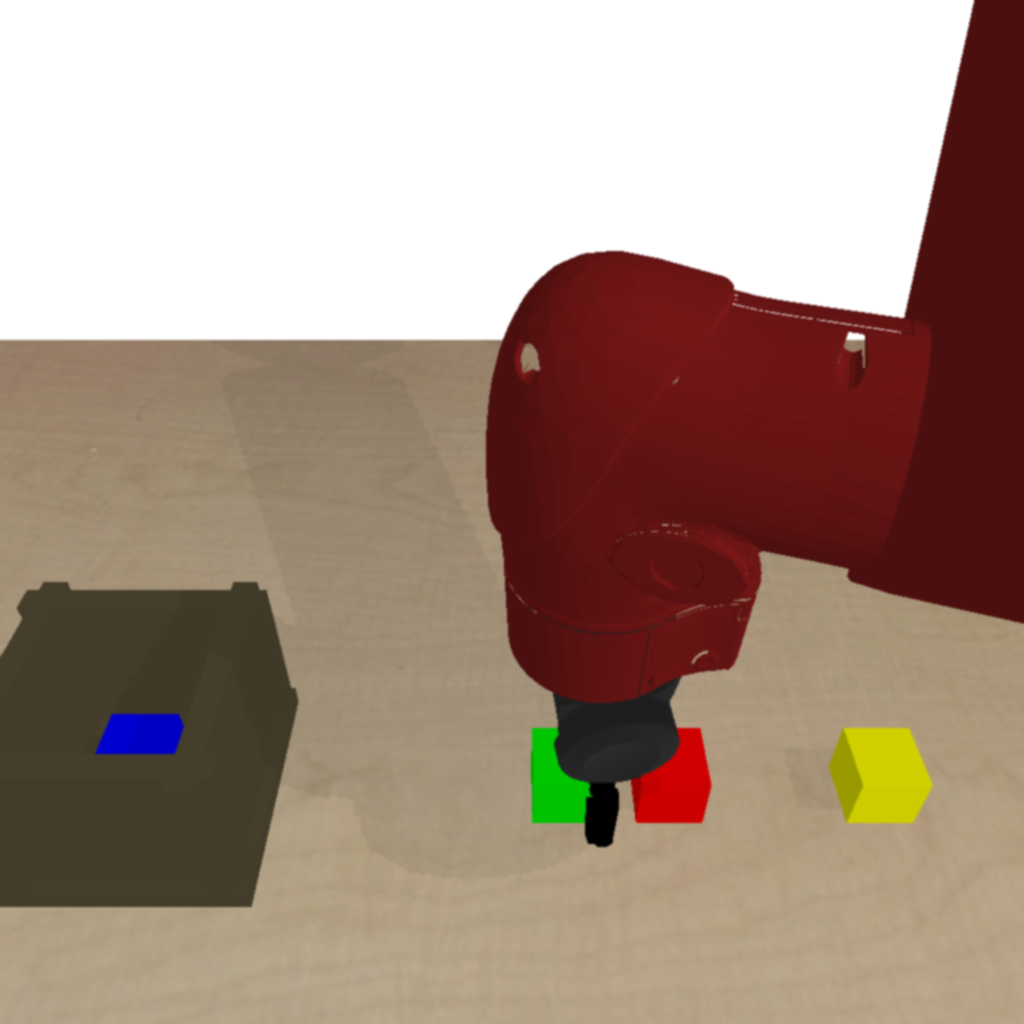}
    \hfill
    \includegraphics[height=2.2cm]{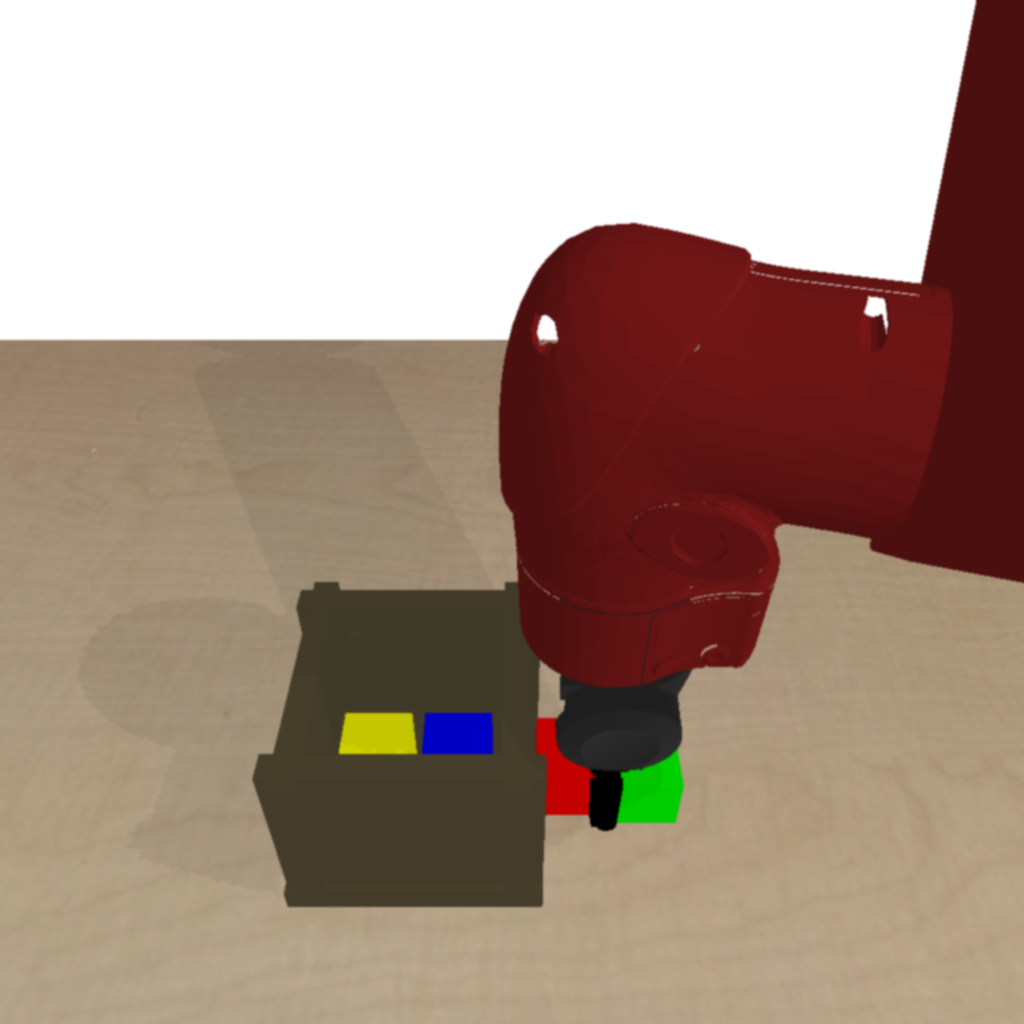}
    \hfill
    \includegraphics[height=2.2cm]{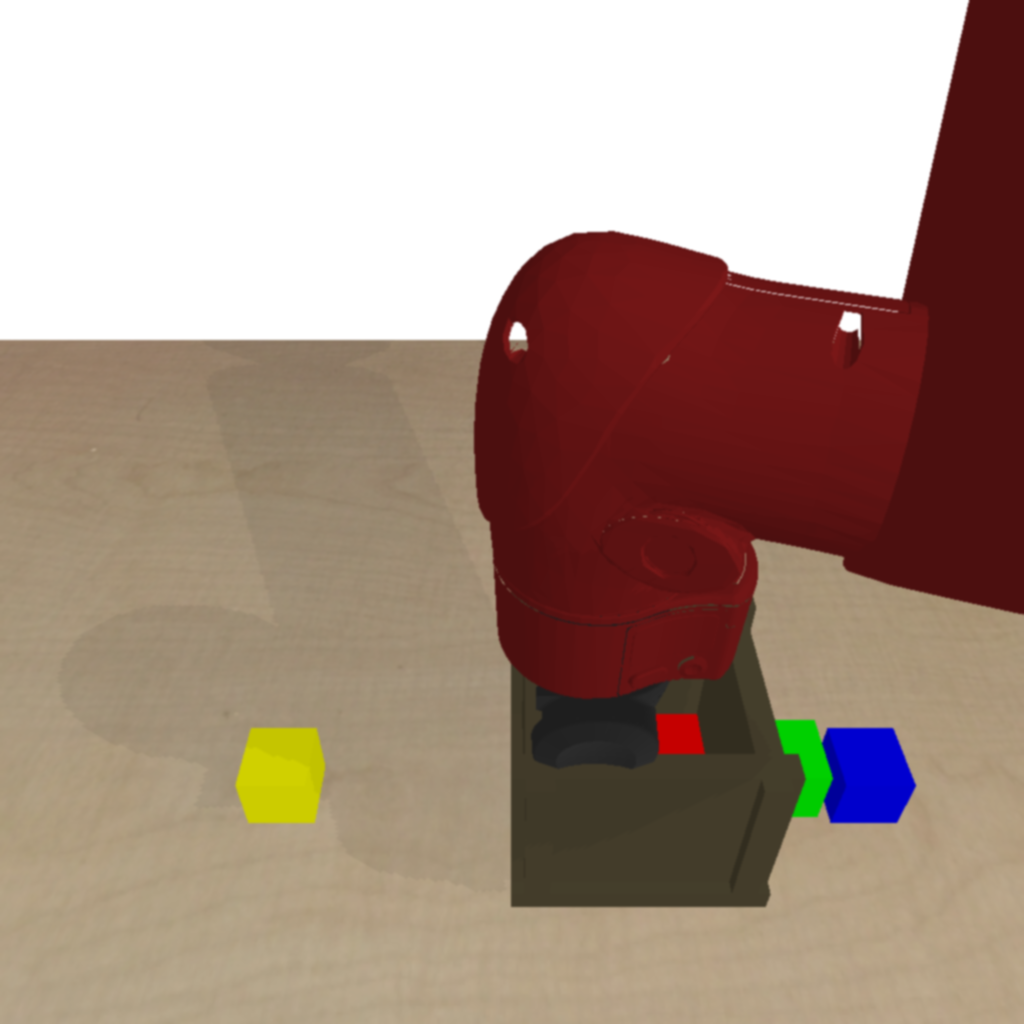}
    \caption{Example images with the hand in a fixed position used to obtain a goal distribution.}
    \label{fig:example-images}
\end{figure}

\paragraph{IKEA}
We adapted this environment from the suite of furniture assembly environments developed by \citet{lee2019ikea}.
In our environment, the agent must learn to attach a set of 3 shelves to a pole.
It can do so by controlling two end effectors: one end effector that can move the pole, and another end effector that can move the shelves.
The former end effector is always attached to the pole, while the latter end effector can selectively attach and detach itself from the shelves.
Both end effectors can move via 3D position control, in a $1 \times 1 \times 1$ area for a maximum of $0.05$ units (in each direction) per timestep.
The end effector interfacing with the shelves can hold onto a shelf by applying a grasp action when it is within the bounding box region of a shelf.
Each shelf has a connection point at which point it will attach to the pole, and the pole has a receiving connection point as well.
When these two connection points are within $0.2$ units away from one another, the shelf automatically attaches to the pole and becomes welded.
The objects have 3 degrees of freedom via translations in 3D space.
The objects are not allowed to collide with one another -- if an action causes them to collide, that action is ignored by the environment and the next state is the same as the current state.
As an exception, when an end effector is not grabbing an object, it is allowed to move through objects.
The agent has access to state information, comprising the 3D position of the end effectors, shelves, and the pole, and indicator information for whether each end effector is grasping an object.

\paragraph{Flat World}
This two-dimensional environment consists of a policy and 4 objects, each of which are defined by their XY-coordinate.
The policy and objects are in an enclosed $8 \times 8$ unit space.
The policy's action space is three dimensional:
two correspond to relative change in position, for a maximum of 1 unit in each dimension per timestep, and one corresponds to a grab action.
The grab action takes on a value between $-1$ and $1$.
If this grab action is positive, then the policy picks up the closest object that is within 1 unit of it, or none if there are no such objects.
If this grab action is non-positive, then the policy drops any object that it was holding.
While an object is grabbed, the object moves rigidly with the policy.
The policy can only grab one object at a time, with ties broken by a predetermined, fixed order.
The agent has access to state information, comprising the 2D position of the policy and the 4 objects.

\section{Experimental Details}\label{appsec:exp-details}

\paragraph{Learning from Examples}
These experiments were evaluated on the Sawyer and FlatWorld environment.
In this section we describe the setup for the Sawyer environment with Gaussian goal distributions.
In this setting, the agent needs to pick up one of the blocks (specifically, the red block) and place it into the tray.
The initial position of the tray and objects vary in each episode.
The objective is only to minimize the relative distance between the red block and the tray, and it is important for the agent to ignore the absolute position of the other blocks and the tray.
The robot can attempt to slide the tray to a specific goal location, but the tray is heavy and moves very slowly. If it successfully moves the tray to another location, it will not have enough time in the episode to move the red block.

We generated $K=30$
examples of successful goal states, in which the red block is always inside the tray, and the tray, other objects, hand, and gripper are in random locations and configurations.
We provided this set of example goal states as input to the competing baselines. Each baseline used the example states in the following manner:
\begin{itemize}
    \item DisCo RL: infer a goal distribution from the example states
    % \item GCRL: the example states are the set of goals for exploration rollouts, and the set of goals sampled for relabeling in training
    \item VICE: a classifier is trained to predict whether a state is optimal, with the example states as the positive examples for the classifier
\end{itemize}
For evaluation, a trajectory is successful if the red block is placed in the tray.
We plot this success metric over time in \autoref{fig:single-task-results}.

\paragraph{Conditional Distributions for Sub-Task Decomposition}
For the multi-task evaluations, we performed experiments in all three of our environments. For each environment, we split the task into several subtasks, as described below:
\begin{itemize}
    \item Sawyer: move the blocks to their goal locations. Each subtask represents moving one block at a time to its goal location.
    \item IKEA: move the pole and the shelves to their goal locations. Each subtask represents moving the pole and one of the shelves to their goal locations.
    \item Flat World: move the objects to their goal locations. Each subtask represents moving one object at a time to its goal location.
\end{itemize}
We generated an example dataset of successful states for each subtask.
For each example state for a particular subtask, we also provided a state representing the final configuration for the entire task (after all subtasks are solved).
See \autoref{sec:disco_impl} for additional details regarding the example sets.
The evaluation metrics for each environment are as follows:
\begin{itemize}
    \item Sawyer: the number of objects that are within $0.10$ units of their respective final goal locations
    \item IKEA: the number of shelves that are connected to the pole, in addition to an indicator for whether the pole is within $0.10$ units of its final goal location 
    \item Flat World: the number of objects that are within $1$ unit of their respective final goal locations
\end{itemize}

For evaluation, we provide the HER baseline oracle goals.
In this setting, the provided goal is identical to the initial state at the beginning of the episode, except for the position of the red block, which we set to be inside the tray.
For example, if the state is given by
\begin{align*}
    \bs_0 = \begin{bmatrix}
    x_0^\text{EE},
    y_0^\text{EE},
    x_0^\text{red-block},
    y_0^\text{red-block},
    x_0^\text{blue-block},
    y_0^\text{blue-block},
    \dots
    % x_0^\text{green-block},
    % y_0^\text{green-block},
    % x_0^\text{yellow-block},
    % y_0^\text{yellow-block},
    \end{bmatrix},
\end{align*}
and we want the red block to move to a position $(x^*, y^*)$, we set the goal to
\begin{align*}
    \bs_g = \begin{bmatrix}
    x_0^\text{EE},
    y_0^\text{EE},
    \textcolor{blue}{
    x^*,
    y^*
    },
    x_0^\text{blue-block},
    y_0^\text{blue-block},
    \dots
    % x_0^\text{green-block},
    % y_0^\text{green-block},
    % x_0^\text{yellow-block},
    % y_0^\text{yellow-block},
    \end{bmatrix}.
\end{align*}
%%GB.8.4: This is still a bit unclear. an we just put the simple math the is performed for the assignment?
In theory, this oracle goal encourages the robot to focus on moving the red block to its goal rather than moving the other state components.
The HER baseline only uses this oracle during evaluation.

Details regarding the distribution of final goal states used for exploration rollouts and relabeling during training, are provided in \autoref{table:env-goals}.
For evaluation, we used $H=100$ for the IKEA and Flat World environments, and $H=400$ for the Sawyer environment.

\begin{table*}[h]
    \vspace{0.25cm}
    \centering
    \begin{tabular}{p{2.25cm}|p{3cm}|p{3cm}|p{2.75cm}}
    \hline
    \textbf{Goal Use Case} & \textbf{Sawyer} & \textbf{IKEA} & \textbf{Flat World}\\
    \hline
    Exploration & $50\%$: objects on ground, $50\%$: objects in tray & Shelves assembled, pole in random position & Objects in random positions\\
    \hline
    Training & Same as above & Objects in random positions & Same as above\\
    \hline
    \end{tabular}
\caption{Environment specific final goal distributions.}
\label{table:env-goals}
\end{table*}

\section{Implementation Details}\label{appsec:implementation-details}

\subsection{General Training Algorithm and Hyperparameters}
In our experiments, we use soft actor-critic as our RL algorithm~\citep{haarnoja2018sac}.
For specific details on the hyperparameters that we used, see \autoref{table:general-hyperparams}.

\begin{table*}
    \centering
    \begin{tabular}{c|c|c|c}
    \hline
    \textbf{Hyper-parameter} & \textbf{Sawyer} & \textbf{IKEA} & \textbf{Flat World}\\
    \hline
    Number of examples (per subtask) $K$ & $30$ & $50$ & $30$\\
    Std. dev. of Gaussian noise added to example set data & $0.01$ & $0.1$ & $0.01$\\
    \hline
    \end{tabular}
\caption{Environment specific hyper-parameters.}
\label{table:env-hyperparams}
\end{table*}

\begin{table*}
    \centering
    \begin{tabular}{c|c}
    \hline
    \textbf{Hyper-parameter} & \textbf{Value}\\
    \hline
    horizon $H$ (for training) & $100$\\
    batch size & $2048$\\
    discount factor & $0.99$\\
    Q-function and policy hidden sizes & $[400, 300]$\\
    Q-function and policy hidden activations & ReLU\\
    replay buffer size & $1$ million\\
    hindsight relabeling probability & $80\%$\\
    target network update speed $\tau$ & $0.001$\\
    number of training updates per episode $N_\text{updates per episode}$ & $100$\\
    number of training batches per environment step & $1$\\
    \hline
    \end{tabular}
\caption{General hyper-parameters used for all experiments.}
\label{table:general-hyperparams}
\end{table*}

\subsection{\METHOD} \label{sec:disco_impl}
\paragraph{Covariance Smoothing}
We apply pre-preprocessing and post-processing steps to obtain the distribution parameters used in RL.
In the pre-processing phase, we add i.i.d. Gaussian noise to the dataset of examples.
The amount of noise that we apply varies by environment -- see \autoref{table:env-hyperparams} for specific details.
After inferring the raw parameters of the Gaussian distribution $\mu$ and $\Sigma$, we apply post-processing steps to the covariance matrix.
We begin by inverting the covariance matrix $\Sigma$.
For numerical stability, we ensure that the condition number of $\Sigma$ does not exceed $100$ by adding a scaled version of the identity matrix to $\Sigma$.
After obtaining $\Sigma^{-1}$, we normalize its components such that the largest absolute value entry of the matrix is $1$.
Finally, we apply a regularization operation that thresholds all values of the matrix whose absolute value is below $0.25$ to $0$.
We found this regularization operation to be helpful when the number of examples provided is low, to prevent the Gaussian model from inferring spurious dependencies in the data.
% We used the resulting $\mu$ and $\Sigma^{-1}$ in \autoref{eq:gaussian-log-prob-reward} for computing the reward.
We used the resulting $\mu$ and $\Sigma^{-1}$ for computing the reward.

\paragraph{Conditional distribution details} \label{sec:appendix-conditional-relabeling}
To obtain the conditional distribution used for relabeling and multi stage planning, we assume that data is given in the form of pairs of states \mbox{$\{(\bs^{(k)}, \bs_f^{(k)})\}_{k=1}^K$}, in which $\bs^{(k)}$ correspond to a state where a sub-task is accomplished when trying to reach the final state $\bs_f$.
% We fit a joint Gaussian distribution, denoted by \mbox{$p_{\bS, \bS_F}(\bs, \bs_f)$}, to these pairs of states.
We fit a joint Gaussian distribution of the form
\begin{align*}
p_{\bS, \bS_f} = 
\gN
\left(
\begin{bmatrix}\mu_\bs \\ \mu_{\bs_f} \end{bmatrix}
,
\begin{bmatrix}
\Sigma_{\bs \bs} & \Sigma_{\bs \bs_f} \\
\Sigma_{\bs_f \bs} & \Sigma_{\bs_f \bs_f} \\
\end{bmatrix}
\right),
\mu_{(\cdot)} \in \R^{\text{dim}(\gS)},
% \Sigma_{\bs\bs}
% \Sigma_{\bs_f \bs}
% \Sigma_{\bs \bs_f}
% \Sigma_{\bs_f \bs_f}
\Sigma_{(\cdot)}
\in \R^{\text{dim}(\gS) \times \text{dim}(\gS)}
% \mu_s \in \R^{|\gS|}
\end{align*}
to these pairs of states using maximum likelihood estimation.
Since the joint distribution $p_{\bS, \bS_f}$ is Gaussian, the conditional distribution $p_{\bS | \bS_f}$ is also Gaussian with parameters $(\mu, \Sigma) = h(\bs_f)$, where $h$ is the standard conditional Gaussian formula:
\begin{align}\label{eq:conditional-relabeling}
h(\bs_f) = \left( 
\underbrace{
\mu_\bs + \Sigma_{\bs \bs_f} \Sigma_{\bs_f \bs_f}^{-1}(\bs_f - \mu_{\bs_f})
}_{\mu}
,
\underbrace{
\Sigma_{\bs \bs} - \Sigma_{\bs \bs_f}\Sigma_{\bs_f \bs_f}^{-1}\Sigma_{\bs_f \bs}
}_{\Sigma}
\right).
\end{align}
In summary, given a final desired state $\bs_f$, we generate a distribution by computing \mbox{$\gdparam = h(\bs_f)$} according to \autoref{eq:conditional-relabeling}.
This conditional distribution also provides a simple way to relabel goal distributions given a reached state $\bs_r$:
we relabel the goal distribution by using the parameters \mbox{$\omega' = h(\bs_r)$}.

\paragraph{Multi-task exploration scheme}
For training, in $50\%$ of exploration rollouts we randomly selected a single subtask for the entire rollout, and in the other $50\%$ of exploration rollouts we sequentially switched the subtask throughout the rollout, evenly allocating time to each subtask.
For switching the subtask, we simply switched the parameters of the subtask $\mu$ and $\Sigma$.
We randomized the order of the subtasks for sequential rollouts.

\paragraph{Relabeling}
We relabel the parameters of the goal distribution $(\mu, \Sigma)$, and the relabeling strategy we use depends on whether we use conditional goal distributions. For non-conditional distributions, we relabel according to the following strategy:
\begin{itemize}
    \item $40 \%$: relabel $\mu$ to a future state along the same collected trajectory
\end{itemize}

For conditional distributions, we relabel according to the following strategy:
\begin{itemize}
    \item $40 \%$: randomly sample $\bs_f$ from the environment 
    \item $40 \%$: relabel $\bs_f$ to a future state along the same collected trajectory
\end{itemize}
For our multi-task experiments, whenever we perform relabeling, we also relabel $\Sigma$. Specifically, we first randomly sample a task from the set of tasks that we have inferred, and relabel $\Sigma$ to the covariance matrix for that task.

\subsection{HER}\label{sec:gcrl_impl}
Our implementation of goal-conditioned RL follows from hindsight experience replay (HER) \cite{andrychowicz2017her}.
Crucially, we perform off-policy RL, in addition to using the relabeling strategies inspired by HER.
When provided a batch of data to train on, we relabel the goals according to the following strategy:
\begin{itemize}
    \item $40 \%$: randomly sampled goals from the environment, or the example sets
    \item $40 \%$: future states along the same collected trajectory, as dictated by HER
\end{itemize}
Unlike HER, which used sparse rewards, we use the Euclidean distance as the basis for our reward function:
\begin{align}\label{eq:gcrl-reward}
    r(\bs, \bs_g) = -\left\lVert \bs - \bs_g \right\rVert
\end{align}
To avoid manual engineering, the space of goals is the same as the space of states.
I.e., the dimension of the goal is the same as that of the state, and the corresponding entries in $\bs$ and $\bs_g$ correspond to the same semantic state features.

\subsection{VICE}\label{sec:vice_impl}
Variational inverse control with events (VICE) is described in~\citet{fu2018variational}. VICE proposes an inverse reinforcement learning method that extends adversarial inverse reinforcement learning (AIRL) \citet{fu2018airl}. Like AIRL, VICE learns a density $p_\theta(s, a)$ using a classification problem. However, unlike the usual IRL setting, VICE assumes access to an example set that specifies the task -- the same assumption as DisCo RL.

VICE alternates between two phases: updating the reward and running RL. To learn a reward function, VICE solves a classification problem, considering the initial example set as positives and samples from the replay buffer as negatives. The discriminator is:
\begin{align}
    D_\theta(s, a) = \frac{p_\theta(s, a)}{p_\theta(s, a) + \pi(a|s)}.
\end{align}
At optimality, the reward recovered $p_\theta(s, a) \propto \pi^*(a|s) = \exp(A(s, a))$, the advantage of the optimal policy~\cite{fu2018airl}.
In practice the reward is represented as $p_\theta(s)$, ignoring the dependence on actions. However, actions are still needed to compute the discriminator logits; we follow the method specified in VICE-RAQ \cite{singh2019raq} to sample actions from $\pi(a|s)$ for all states. We also use mixup \cite{zhang2018mixup} as described in VICE-RAQ. Mixup significantly reduces overfitting and allows VICE to successfully learn a neural net classifier even with so few (30 to 50) positive examples. In the RL phase, VICE runs reinforcement learning with $\log p_\theta(s, a)$ as the reward function, actively collecting more samples to use as negatives.

We re-implemented VICE as above and confirmed that it successfully learns policies to reach a single state, specified by examples. However, our results demonstrate that VICE struggles to reach the example sets we use in this work. This issue is exacerbated when the problem is multi-task instead of single-task and the state includes a goal, as in goal-conditioned learning.

In multi-stage tasks, we train a single DisCo RL policy shared among the stages. For VICE, sharing data among different tasks would not respect the adversarial optimization performed by the method. Instead, we train separate policies for each stage without sharing data between policies. Thus, for a task with $N$ stages, VICE is generously allowed to experience $N\times$ the data, as each policy collects its own experience).
